# Supplementary material for: Appearance Matching Adapter for Exemplar-based Semantic Image Synthesis in-the-Wild
Source: arXiv:2412.03150 source file (2025-03-18)
Supplement: Supplementary file 1 [file cross_domain_setting.tex]

\begin{figure*}[t]
    \centering
    \includegraphics[width=\textwidth]{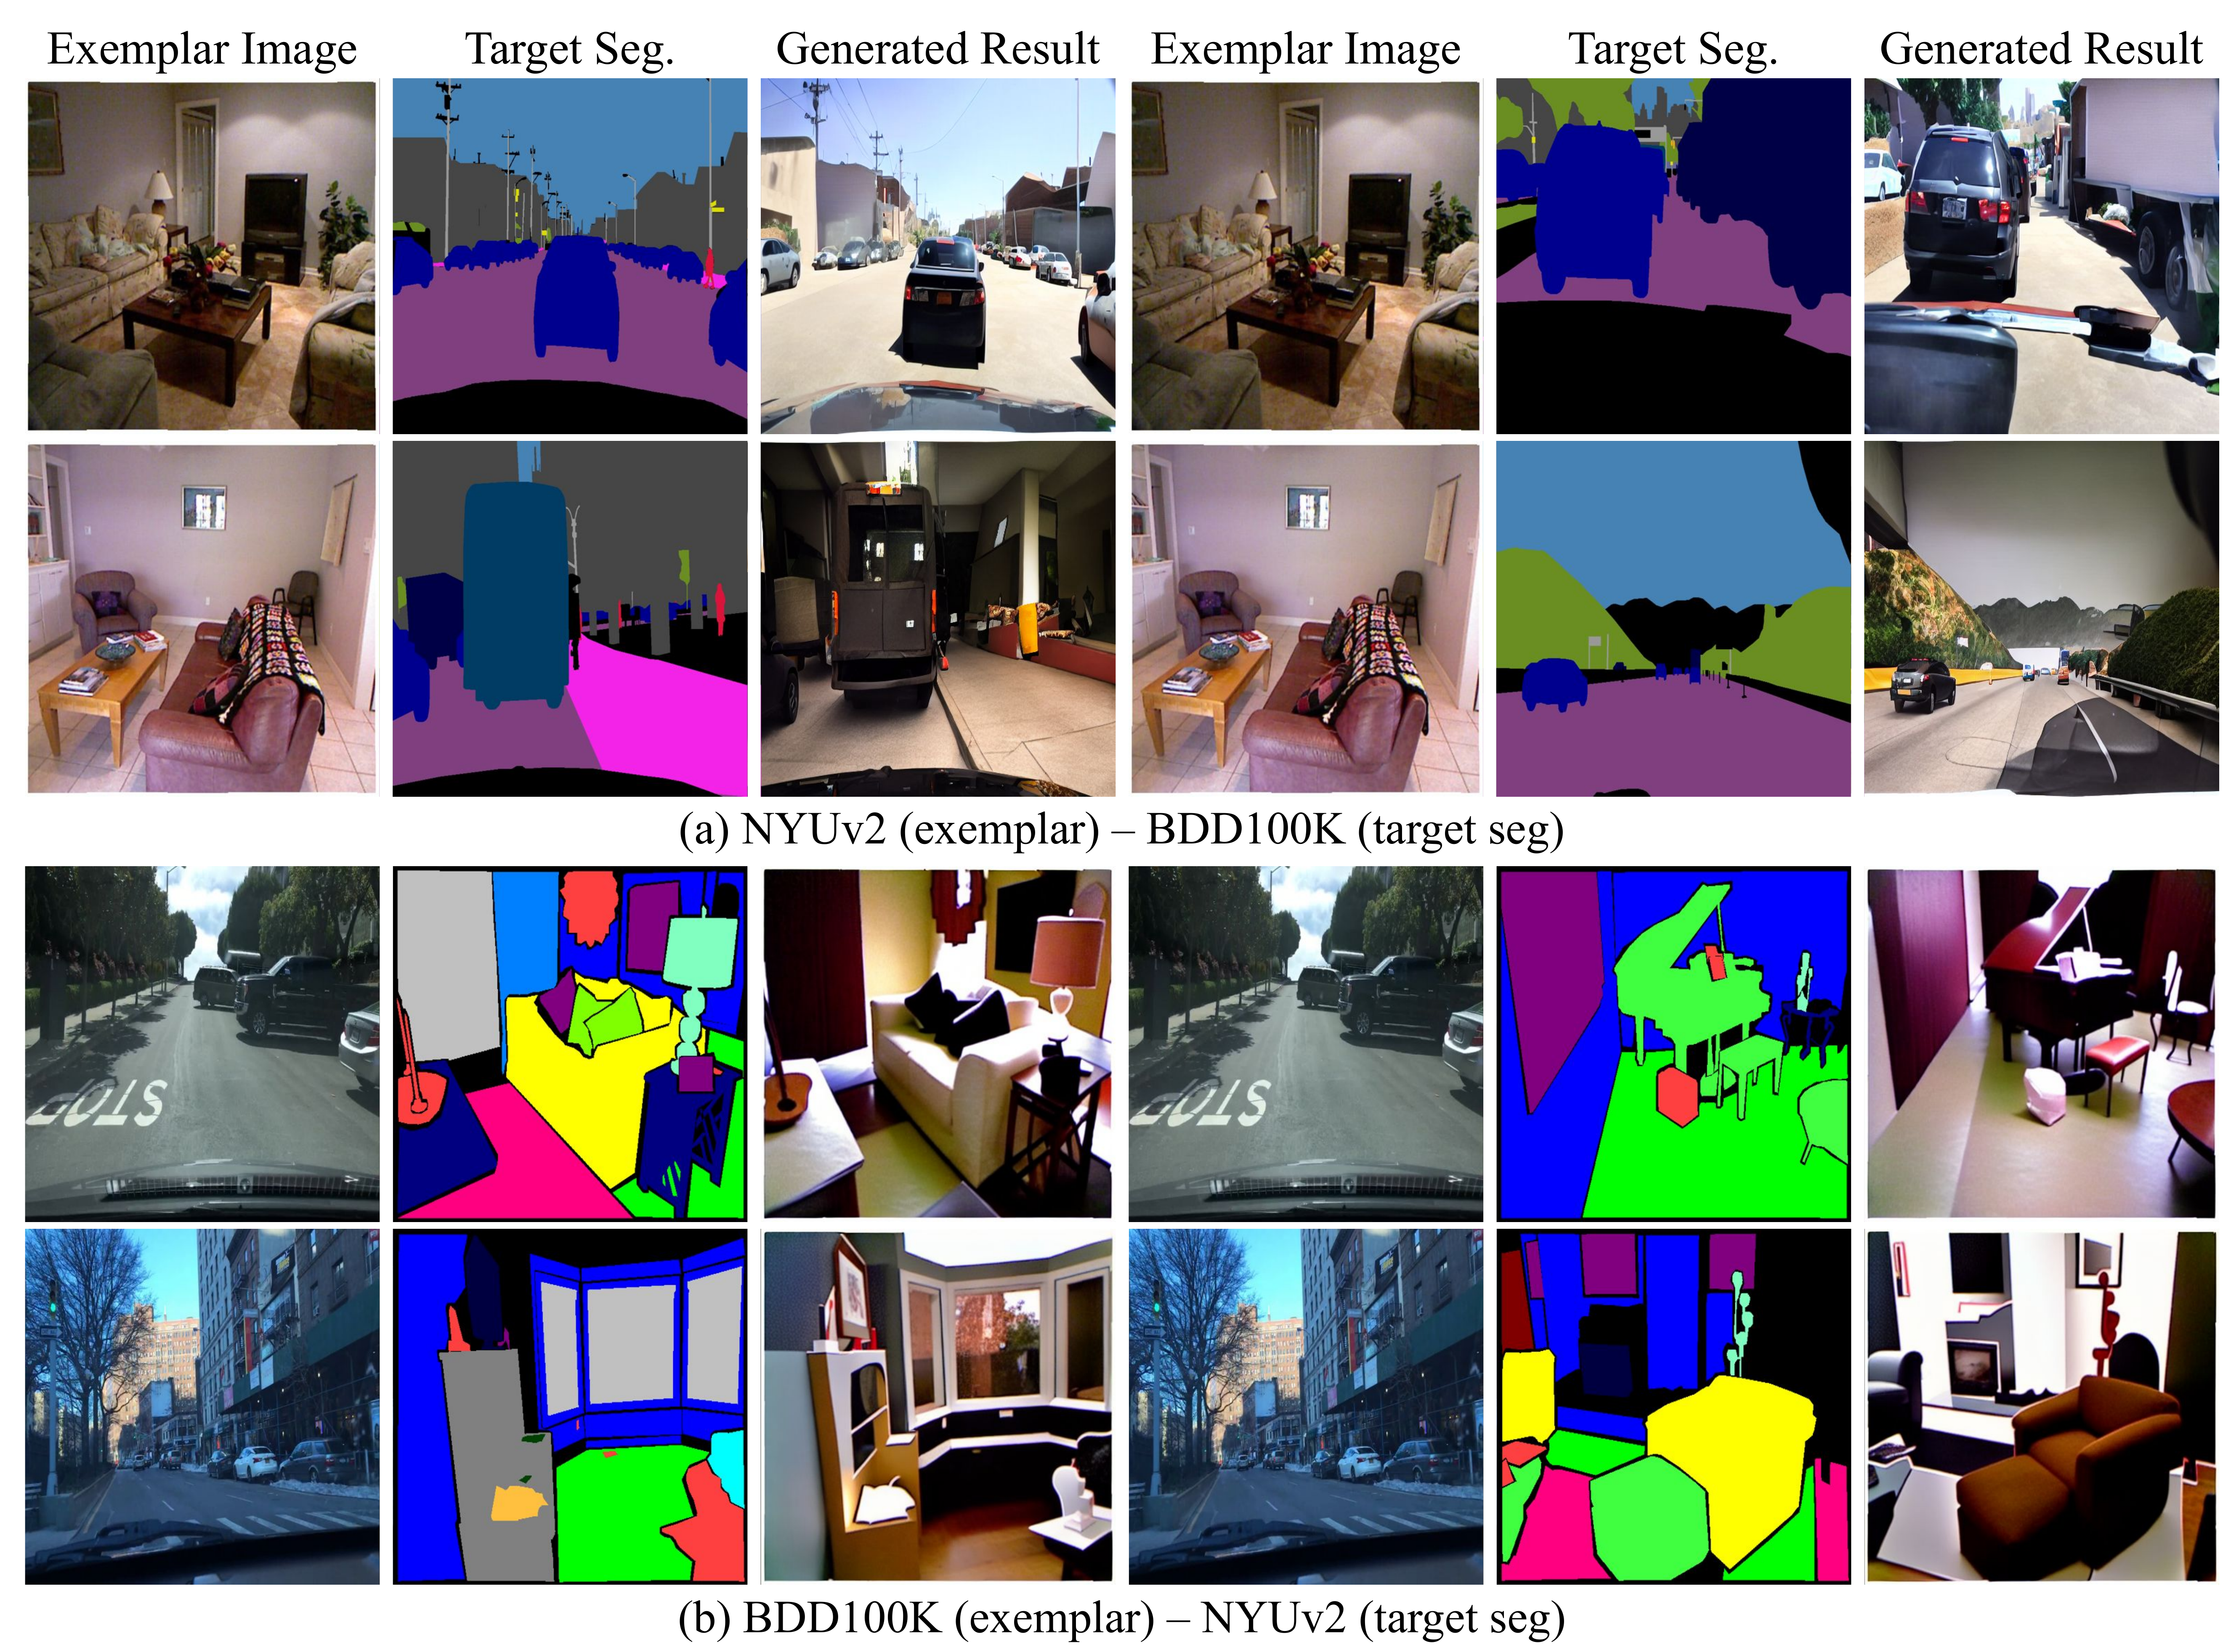} 
    \vspace{-20pt}
    \caption{\textbf{Cross Domain Setting.}}
    \vspace{-10pt}
    
    \label{supple:cross_domain}
\end{figure*}
