# Supplementary material for: Appearance Matching Adapter for Exemplar-based Semantic Image Synthesis in-the-Wild
Source: arXiv:2412.03150 source file (2025-03-18)
Supplement: Supplementary file 2 [file dino_table.tex]

\begin{table*}[t]
\small
% \centering
\resizebox{\linewidth}{!}{
    \begin{tabular}{l|cc|ccc|c|c}
    \toprule
    % \multirow{2}{*}{Methods} & \multirow{2}{*}{Training} & \multicolumn{4}{c|}{BDD100K~\cite{yu2020bdd100k}} \\
    \cmidrule(lr){3-9} BDD100K Comparison & ControlNet & ControlNeXt & FreeControl & Cross-Image Attention & Ctrl-X & ControlNet + IP-Adapter & \textbf{AM-Adapter(Ours)} \\
    
    %Self-sim $\downarrow$ & $I_{\mathrm{DINO}}$ $\uparrow$ & $I_{\mathrm{CLIP}}$ $\uparrow$  &CLIP-FID $\downarrow$ \\
    % \cmidrule(lr){3-5}\cmidrule(lr){6-8}
    \midrule

    DINO [CLS] loss $\downarrow$ & 0.095 & 0.078 & 0.100 & 0.137 & \cellcolor{warmyellow}{0.063} & 0.072 & \textbf{\cellcolor{yzybest}{0.056} } \\
    $I_\text{DINO}$ $\uparrow$ & 0.654 & 0.695 & 0.479 & 0.495 & \cellcolor{warmyellow}{0.743} & 0.732 & \textbf{\cellcolor{yzybest}{0.765}} \\
    % Ctrl-X~\cite{lin2024ctrl}  &  0.051 & \cellcolor{yzybest}{0.788} & 0.700  & 45.75  \\

    % ControlNet~\cite{zhang2023adding} + IP Adapter~\cite{ye2023ip} & \cellcolor{warmyellow}{0.049} & 0.759 & \cellcolor{warmyellow}{0.805} & \cellcolor{yzybest}{15.35}  \\

    % \midrule
    % \bluerow \textbf{AM-Adapter (Ours)} &  \cellcolor{yzybest}{0.041} & \cellcolor{warmyellow}{0.786} & \cellcolor{yzybest}{0.819} & \cellcolor{warmyellow}{16.66}  \\
    \bottomrule
    \end{tabular}
    }
% \vspace{-5pt}
% \caption{\textbf{Quantitative comparisons.}}
% \label{tab:metric}
% \vspace{-10pt}
\end{table*}
